# Supplementary material for: The magneto-structural relationship in the tetrahedral spin chain oxide CsCoO$_2$
Source: arXiv:1410.3686 source file (2014-10-14)
Supplement: Supplementary file 1 [file SI-submission1.pdf]

# Supplemental Information:
# The magneto-structural relationship in the tetrahedral spin chain oxide $CsCoO_2$

N. Z. Ali,[1] R. C. Williams,[2] F. Xiao,[2] S. J. Clark,[2] T. Lancaster,[2] S. J. Blundell,[3] D. V. Sheptyakov,[4] and M. Jansen[1]
[1]*Max-Planck-Institut für Festkörperforschung, Heisenbergstr. 1, D-70569 Stuttgart, Germany*
[2]*Durham University, Department of Physics, South Road, Durham, DH1 3LE, UK*
[3]*Oxford University Department of Physics, Parks Road, Oxford, OX1 3PU, UK*
[4]*Laboratory for Neutron Scattering and Imaging,*
*Paul Scherrer Institut, CH-5232 Villigen, Switzerland*
(Dated: October 13, 2014)

## I. FURTHER EXPERIMENTAL DETAILS

$CsCoO_2$ was synthesized along the Azide/Nitrate Route, details of the procedure have been reported elsewhere.[1,2]

Differential scanning calorimetry (DSC) measurements on a polycrystalline sample of $CsCoO_2$ were carried out with a DSC device (DSC 404 C, Netzsch GmbH, Selb, Germany) operating in a heat flux mode. The polycrystalline sample is exposed to a linear temperature program and heated at a rate of 10 K/min under streaming dry argon gas up to 600 K. Background contributions were subtracted using external sapphire calibrations. A series of measurements were made consecutively at regular intervals employing an aluminium crucible with a lid, to achieve high reproducibility and precision.

Neutron powder diffraction (NPD) measurements were made on approximately 2 g of polycrystalline $CsCoO_2$ powder (obtained from six individual batches), enclosed using a graphite sealing in a vanadium cylindrical sample container with diameter of $\approx 6$ mm under helium atmosphere. NPD measurements were made with the High Resolution Powder Diffractometer for Thermal Neutrons, HRPT[3] at SINQ spallation neutron source, at temperatures ranging from 1.5 to 700 K.

For the temperatures below room temperature (1.5–270 K), a standard orange cryostat was used, the intermediate temperature patterns (at 210–330 K) were collected using the closed-cycle refrigerator with an additional heating stage, while for the temperatures above room temperature, a radiation-type furnace was used. Altogether, 5 different set-ups of the instrument optics and sample environment configuration were used.

Data were collected with the high resolution powder diffractometer HRPT[3] at the SINQ spallation source for $1.5 \leq T \leq 700$ K. Lattice constants, atomic coordinates and hence interatomic distances and angles were systematically refined for all the NPD datasets. At several selected temperatures $(1.5, 300, 480$ and $700$ K) high intensity datasets were collected in order to precisely refine all structural parameters. The structural parameters obtained using Rietveld refinement are consistent with those previously reported, which were obtained using single crystal x-ray scattering.[1] At 1.5, 300, 480 and 700 K high intensity datasets were collected in order to precisely refine all structural parameters. These highest quality datasets always comprised at least one collection with high intensity mode and neutron wavelength $\lambda = 1.494$ Å, and one dataset collected in the medium resolution mode and $\lambda = 1.886$ Å. At all other intermediate temperatures, the data were collected with a neutron wavelength $\lambda = 1.886$ Å and high intensity mode of HRPT. The refinements of the parameters of crystal and magnetic structures were carried out with the FULLPROF suite of programs[4], with the use of its internal tabulated values of the coherent elastic neutron scattering lengths (5.42, 2.49 and 5.803 fm for Cs, Co and O respectively), as well as of the magnetic neutron scattering form-factors for the magnetic $Co^{3+}$ ion.

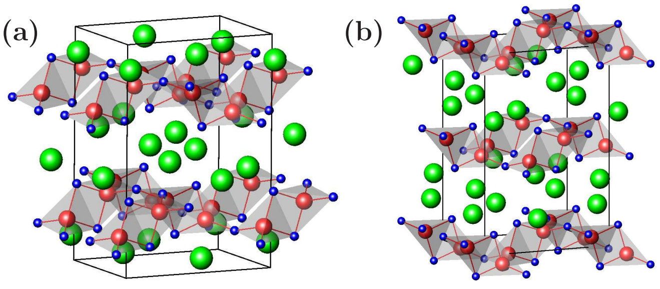

FIG. S1. Illustration of the nuclear structure of $CsCoO_2$, depicting (a) the low-temperature monoclinic $\alpha$ phase structure refined at 2 K and (b) the high-temperature orthorhombic $\beta$ phase refined at 300 K.

Fig. S1 provides illustrations of the nuclear structures for both the $\alpha$ (low temperature, monoclinic) and $\beta$ (high temperature, orthorhombic) phases of $CsCoO_2$, containing two and three $CoO_2$ layers respectively, as refined from the NPD data. Fig. S2 displays examples of the Rietveld refinement fits carried out on the higher statistics datasets. The polycrystalline powder of $CsCoO_2$ contains traces of cobalt(II) oxide, CoO,[5–7] and metallic silver[8] particles from the autoclave as an impurity. The impurity contents remained constant ($< 5\%$) throughout the analysis, as controlled by the multi-phase Rietveld refinement procedures.

The Rietveld refinement of the NPD patterns acquired in the temperature range $1.5 < T < 100$ K, in space group $C2/c$, using the atomic coordinates of $\alpha$-$CsCoO_2$ as the starting model,[1] show a satisfactory agreement between the experimental and calculated nuclear Bragg

peaks, [see Fig. S2(a, b)]. The superior quality of refinement for datasets collected using $\lambda = 1.494$ Å may be seen by comparing these plots. The neutron diffraction patterns collected between $100 < T < 700$ K are consistent with orthorhombic $Cmca$ symmetry and may also be correctly fitted employing the structural model proposed earlier via our single crystal x-ray measurements.[1] The good agreement between the calculated and observed patterns is presented in Fig. S2(c). Refined crystal structure parameters (together with bond distances and angles) for both phases of $CsCoO_2$ are presented in table S1, as obtained using high intensity NPD. Atomic coordinates and isotropic thermal displacement parameters for $\beta$- and $\alpha$-$CsCoO_2$ are presented in tables S2 and S3 respectively.

Below $T^\star \approx 100$ K, the displacive structural phase transition from monoclinic $Cmca$ ($\beta$ phase) to monoclinic $C2/c$ ($\alpha$ phase) is observed, producing a set of new reflections and splitting of certain nuclear intensities accompanying the lowering of symmetry.

The Co-O1 bond distance in $Co_2O_6$ anions bridging over the O1-O1 edge is slightly larger than the corresponding Co-O2,O3 bond distances bridging through corners, owing to the inter-cationic repulsion across the Co-Co junction in $Co_2O_6$ anions. This structural distortion, accompanied by the monoclinic angle of 92°, result in a significant tilting of the corner connected $Co_2O_6$ dimeric units leading to systematic dovetail twin in $\alpha$-$CsCoO_2$, as reported exclusively in our recent single crystal diffraction study.[1] This displacive structural phase transition is, however, relevant for the magnetic exchange coupling within the ${}^2_\infty CoO_2$ polyanion.

Fig. S3 shows the temperature-dependence of the ordered moment size of the cobalt ions below $T_N$, as refined from the NPD data.

### A. Density Functional Theory

The density functional plane wave pseudopotential method within the generalized gradient approximation was used as implemented in the CASTEP code.[9,10] The plane wave basis set (kinetic energy cutoff and $k$-point sampling) was set such that total energy differences were converged to better than 1 meV/unit cell. The PBE-GGA functional was used for both valence electrons and to generate the ultrasoft pseudo potentials. A systematic search was performed to categorize the possible AFM structures.

### B. Muon Spin Rotation

Zero-field (ZF) $\mu$SR measurements were made using the GPS instrument at the Swiss Muon Source. The $CsCoO_2$ powder was loaded into a titanium sample holder in an argon-filled glovebox, covered with 25 $\mu$m Ti foil and made air-tight with a knife edge seal. In a $\mu^+$SR experiment,[11] spin-polarized positive muons are implanted into the sample and subsequently decay into a positron with average lifetime $\tau = 2.2$ $\mu$s. The decay positron is emitted preferentially in the direction of the muon's instantaneous spin vector. Detectors grouped Forward (F) and Backward (B) with respect to the muon beam's initial spin polarization direction allow one to measure the positron asymmetry

$$A(t) = \frac{N_\mathrm{F}(t) - \alpha N_\mathrm{B}(t)}{N_\mathrm{F}(t) + \alpha N_\mathrm{B}(t)}, \tag{1}$$

where $N_\mathrm{F,B}(t)$ are the event histograms at a time $t$ after the muon implantation, and $\alpha$ is an experimental calibration constant. The asymmetry $A(t)$ is proportional to the muon ensemble's spin polarization, the time-dependence of which is sensitive to the local magnetic field experienced at the muons' stopping sites. The Larmor precession frequency of the muon ensemble is related to the average magnitude of the static magnetic field $B$ at the muon site via $2\pi\nu = \gamma B$. Here $B$, and hence $\nu$ serves as an effective order parameter for the LRO.

The dipolar field $\mathbf{B}_\mathrm{dip}(\mathbf{r}_\mu)$ at the muon site $\mathbf{r}_\mu$ due to the coupling with localised magnetic moments $\mathbf{m}_i$ located at positions $\mathbf{r}_i$ is given by

$$\mathbf{B}_\mathrm{dip}(\mathbf{r}_\mu) = \frac{\mu_0}{4\pi} \sum_i \frac{3(\mathbf{m}_i \cdot \hat{\mathbf{r}}_{i\mu})\hat{\mathbf{r}}_{i\mu} - \mathbf{m}_i}{|\mathbf{r}_\mu - \mathbf{r}_i|^3}, \tag{2}$$

where $\mu_0$ is the vacuum permeability, $\hat{\mathbf{r}}_{i\mu}$ the normalised vector between the muon and the moment $\mathbf{m}_i$. The dipolar interaction may be evaluated for an infinite sample by calculating the magnetic field given by Eq. 2 within a Lorentz sphere of finite radius $r_\mathrm{L}$. The Lorentz sphere needs to be sufficiently large to reach satisfactory convergence of the calculated field. In our calculations $r_\mathrm{L} = 42$ Å. As only antiferromagnetic structures were considered, no further terms need to be considered for the diamagnetic muon sites.

If the magnetic field experienced by the muon is entirely dipolar (i.e. we neglect the contact hyperfine field) then the magnetic field calculated at any given site is proportional to the precession frequency of a muon situated there. Therefore we may obtain the frequency (per unit moment size) probability density function (PDF) $f(\nu/\mu)$, both for the entire unit cell, and for a reduced volume fraction satisfying physically justified constraints on muon sites. The constraints applied were that a muon typically lies 1 Å away from an oxygen ion[12] ($0.9 \leq r_1 \leq 1.1$ Å) and won't come to rest too close a positively charged ion ($r_2 \geq 1$ Å). Using Bayesian inference together with the observed precession frequency,[13] one is able to find the PDF for the ordered moment size using

$$g(\mu|\nu) = \frac{\frac{1}{\mu} f(\nu/\mu)}{\int_0^{\mu_\mathrm{max}} \frac{1}{\mu'} f(\nu/\mu')\,\mathrm{d}\mu'}, \tag{3}$$

where the prior moment size distribution has been taken to be a uniform probability between zero and $\mu_{\max}$ (calculations are insensitive to the value chosen as long as it exceeds any conceivable value deduced by prior reasoning, which here is $10\mu_{\rm B}$).

The observed precession frequency [Fig. 4(c) in main text] at both 50 K ($\alpha$ phase) and 300 K ($\beta$ phase) was 23.4 MHz. Neutron data indicates that the ordered moment size is $2.63\mu_{\rm B}$ at 296 K, and hence this value was used to scale the frequency PDF shown in Fig. S4(a). The observed frequency $\nu = 23.4$ MHz is labelled, and the PDF has a clear peak lying very close to this value. Using this value of ordered moment size, a candidate muon site was located which lies approximately 1 Å from the corner-sharing oxygen ions, on the outside of the Co-O-Co angle, which would give rise to the observed muon precession frequency. The ordered moment size PDFs $g(\mu|\nu)$ are displayed in Fig. S4(b), and there are peaks positioned very close to the indicated moment size of $2.63\mu_{\rm B}$ within both the $\alpha$ and $\beta$ phases. The fact that all PDFs generated are remarkably similar for the monoclinic $\alpha$ and orthorhombic $\beta$ phases suggests that the impact of the structural transition on the muon stopping site location (and hence local magnetic field strength) is not severe, and is therefore unlikely to be the sole cause of the suppression of the order parameter observed around $T^{\star}$.


[1] N. Z. Ali, J. Nuss, R. K. Kremer, and M. Jansen, Inorg. Chem. **51**, 12336 (2012).

[2] M. Jansen, Z. Anorg. Allg. Chem. **638**, 1910 (2012).

[3] P. Fischer, G. Frey, M. Koch, M. Knnecke, V. Pomjakushin, J. Schefer, R. Thut, N. Schlumpf, R. Brge, U. Greuter, S. Bondt, and E. Berruyer, Physica B **146**, 276 (2000), [http://sinq.web.psi.ch/hrpt].

[4] J. Rodríguez-Carvajal, Physica B **192**, 55 (1993).

[5] G. Natta and A. Reina, An. Fis. Quim. **24**, 611 (1926).

[6] W. Jauch, M. Reehuis, H.J. Bleif, and F. Kubanek, Phys. Rev. B **64**, 052102 (2001).

[7] K. Tomiyasu, T. Inami, and N. Ikeda, Phys. Rev. B **70**, 184411 (2004).

[8] I. K. Suh, H. Ohta, and Y. Waseda, J. Mater. Sci. **23**, 757, (1988).

[9] S. J. Clark, M. D. Segall, C. J. Pickard, P. J. Hasnip, M. I. J. Probert, K. Refson and M. C. Payne, Z. Kristallogr. **220**, 567 (2005).

[10] P. J. Hasnip, K. Refson, M. I. J. Probert, J. R. Yates, S. J. Clark and C. J. Pickard, Phil. Trans. R. Soc. A **372**, 20130270 (2014).

[11] S. J. Blundell, Contemp. Phys. **40**, 175 (1999).

[12] J. H. Brewer *et al.*, Hyperfine Interact. **63**, 177 (1991).

[13] S. J. Blundell, A. J. Steele, T. Lancaster, J. D. Wright and F. L. Pratt, Physics Procedia **30**, 113 (2012).

TABLE S1. Refined crystal structure parameters, as well as the Co-O bond lengths and Co-O-Co bond angles, of $CsCoO_2$ refined in space group $C2/c$ at 1.5 K, and in space group $Cmca$ at 300, 480 and 700 K.

| | 1.5 K | 300 K | 480 K | 700 K |
|---|---|---|---|---|
| Lattice parameters: | | | | |
| $a$ (Å) | 5.9747(2) | 5.9936(2) | 6.0028(3) | 6.0084(4) |
| $b$ (Å) | 12.2045(5) | 12.2529(4) | 12.3177(6) | 12.4243(8) |
| $c$ (Å) | 8.2324(3) | 8.2735(3) | 8.3077(4) | 8.3532(5) |
| $\beta$ (°) | 91.9416(8) | | | |
| Bond lengths and angles: | | | | |
| Co-O1 bonds (Å) (bridging over the O1-O1 edge) | 1.885(4) and 1.878(5) | 1.879(5) and 1.910(5) | 1.894(6) and 1.912(7) | 1.881(7) and 1.905(7) |
| Co-O2.O3 bonds (Å) (bridging through the corners) | 1.826(4) and 1.825(4) | $2 \times 1.811(3)$ | $2 \times 1.805(3)$ | $2 \times 1.814(3)$ |
| Co-Co intradimer (Å) | 2.576(7) | 2.628(6) | 2.653(7) | 2.633(8) |
| Co-Co interdimer (Å) | 3.433(6) and 3.565(6) | 3.495(3) | 3.488(4) | 3.510(4) |
| Co-O1-Co angles (°) (bridging over the edge) | 86.4(3) | 87.9(3) | 88.4(4) | 88.1(5) |
| Co-O2-Co angles (°) (bridging through the corner) | 140.1(4) | 149.6(2) | 150.1(3) | 150.8(3) |
| Co-O3-Co angles (°) (bridging through the corner) | 155.3(4) | | | |

TABLE S2. Atomic coordinates and isotropic thermal displacement parameters for $\beta$-$CsCoO_2$ at selected temperatures.

| | | 300 K | 480 K | 700 K |
|---|---|---|---|---|
| Atom, site: | | | | |
| Cs, $8f(0, y, z)$, | $y$ | 0.3361(2) | 0.3365(2) | 0.3354(2) |
| | $z$ | 0.0733(3) | 0.0753(4) | 0.0733(5) |
| | B (Å$^2$) | 1.29(5) | 2.05(6) | 3.42(9) |
| Co, $8f(0, y, z)$, | $y$ | 0.0489(4) | 0.0479(5) | 0.0469(5) |
| | $z$ | 0.1413(5) | 0.1430(6) | 0.1413(7) |
| | B (Å$^2$) | 1.00(7) | 1.81(9) | 2.74(13) |
| O1, $8f(0, y, z)$, | $y$ | 0.0999(2) | 0.0996(2) | 0.0988(2) |
| | $z$ | $-0.0726(3)$ | $-0.0716(4)$ | $-0.0703(4)$ |
| | B (Å$^2$) | 1.36(5) | 2.04(6) | 2.95(7) |
| O2, $8f(\frac{1}{4}, y, \frac{1}{4})$, | $y$ | 0.0874(2) | 0.0857(3) | 0.0837(3) |
| | B (Å$^2$) | 1.70(5) | 2.63(7) | 3.87(9) |

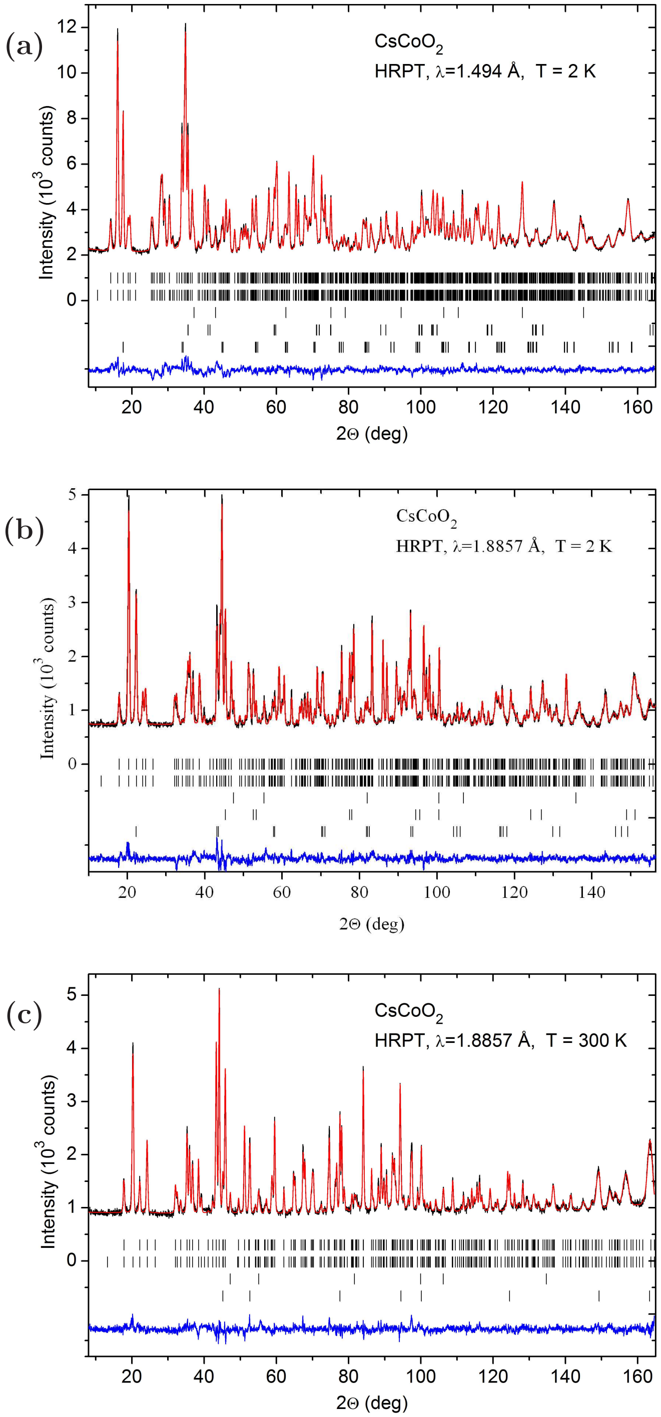


FIG. S2. Rietveld refinements of the crystal and magnetic structure of $CsCoO_2$ at (a, b) 2 K (space group $C2/c$) and (c) 300 K (space group $Cmca$), from NPD data collected with (a) $\lambda = 1.494$ Å in the high resolution mode and (b, c) $\lambda = 1.8557$ Å in the medium resolution mode. The observed intensity, calculated profile and difference curves are shown. The rows of ticks at the bottom of each panel correspond to the calculated diffraction peak positions of the phases (from top to bottom): relevant $CsCoO_2$ nuclear structure, its magnetic phase ($\boldsymbol{k} = 0$), Ag impurity, CoO impurity nuclear structure [monoclinic in (a, b) and cubic in (c)], the magnetic structure of CoO [$\boldsymbol{k} = (0, 1, 1/2)$ in (a, b) only].

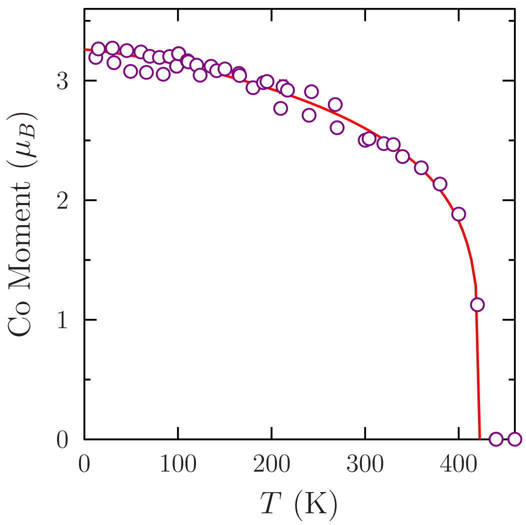


FIG. S3. Ordered $Co^{3+}$ moment size as obtained by Rietveld refinements of NPD data. The solid line is a guide to the eye.

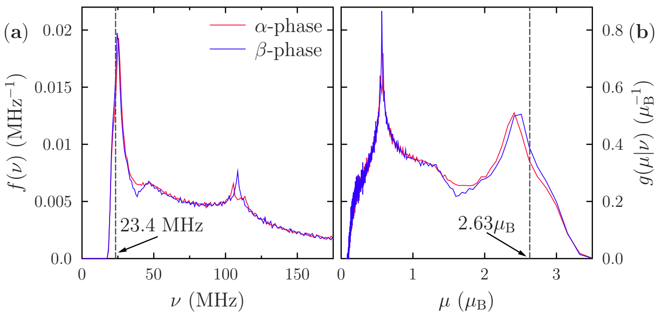


FIG. S4. (a) Precession frequency PDF (scaled for an ordered moment size $\mu = 2.63\mu_B$). (b) Ordered moment size PDF, obtained using the observed precession frequency $\nu = 23.4$ MHz. Data are constrained to a limited volume fraction of the unit cell, as described in the text.

TABLE S3. Atomic coordinates and isotropic thermal displacement parameters for $\alpha$-$CsCoO_2$ refined at 1.5 K.

| Atom, site: | | |
|---|---|---|
| Cs, $8f(x, y, z)$, | $x$ | 0.2556(4) |
| | $y$ | 0.0868(2) |
| | $z$ | 0.5722(3) |
| | $B$ (Å$^2$) | 0.13(4) |
| Co, $8f(x, y, z)$, | $x$ | 0.2487(7) |
| | $y$ | 0.2981(3) |
| | $z$ | 0.8607(6) |
| | $B$ (Å$^2$) | 0.27(6) |
| O1, $8f(x, y, z)$, | $x$ | 0.2438(4) |
| | $y$ | 0.1499(2) |
| | $z$ | 0.9245(3) |
| | $B$ (Å$^2$) | 0.22(3) |
| O2, $4e(0, y, \frac{1}{4})$, | $y$ | 0.6508(3) |
| | B (Å$^2$) | 0.21(5) |
| O3, $4e(0, y, \frac{1}{4})$, | $y$ | 0.1699(3) |
| | B (Å$^2$) | 0.46(6) |
